# Supplementary material for: Electron-mediated anharmonicity and its role in the Raman spectrum of graphene
Source: arXiv:2410.23791 ancillary file (2025-04-30)
Supplement: Supplementary file 1 [file SI.pdf]

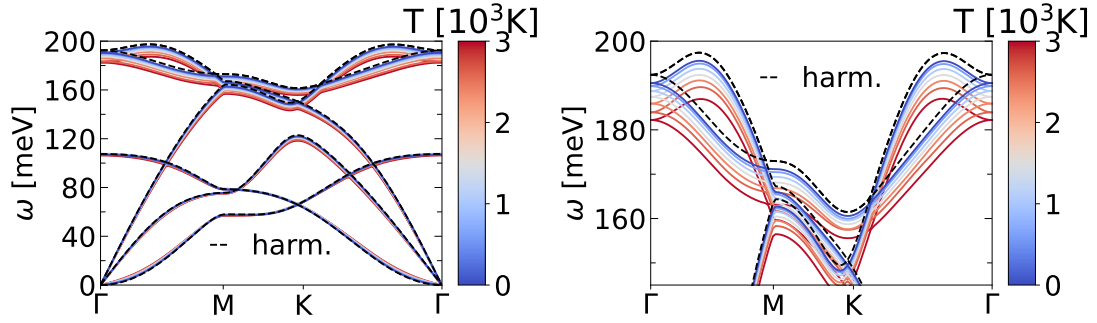

**Supplementary Figure 1.** Graphene phonon dispersion for various temperatures as obtained from SSCHA. Right panel is a close-up of the left panel, highlighting the modifications of the relevant optical phonons.

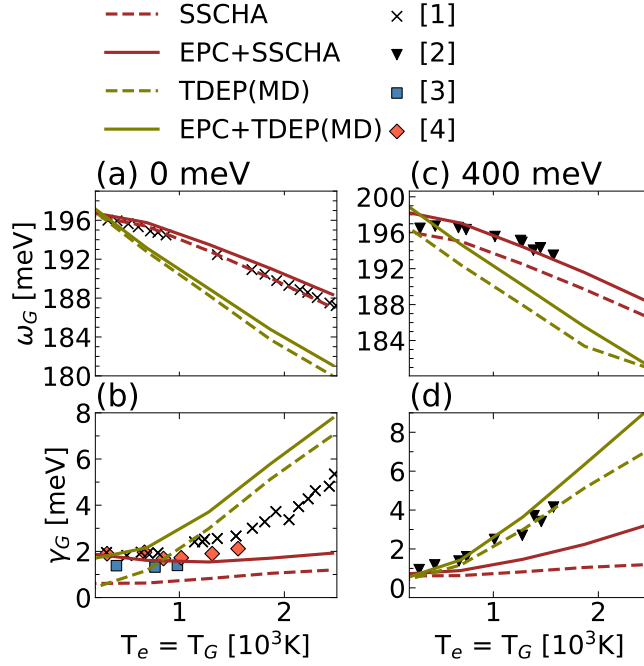

**Supplementary Figure 2.** For the two different doping regimes, we show the total EPC and anharmonicity induced G mode frequency renormalization (a,c) and linewidth (b,d) on the smaller temperature range. We compare anharmonic effects obtained with TDEP with MD and with SSCHA. (a,c) Anharmonic effects have a prevailing temperature dependence at smaller temperatures shown here and determine the G mode frequency decrease with temperature observed in experiments [1, 2]. (b,d) Linewidth increase with temperature observed in Ref. [1–4].

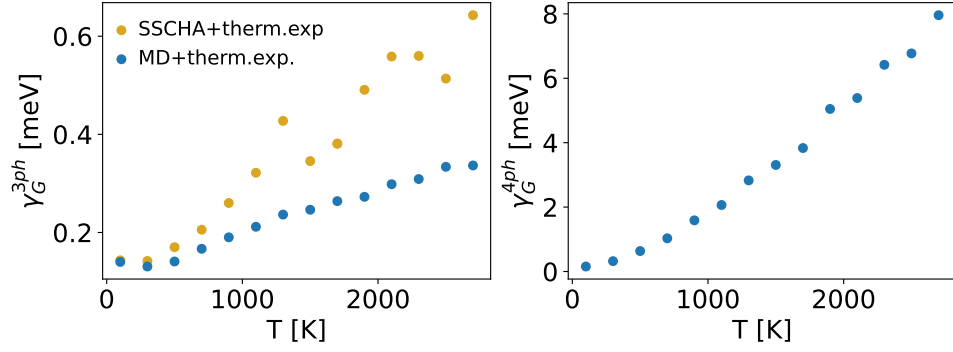

**Supplementary Figure 3.** Comparison between a three-phonon anharmonic contribution to the linewidth as obtained from SSCHA and from TDEP(MD) with a much larger four-phonon contribution obtained from TDEP(MD).

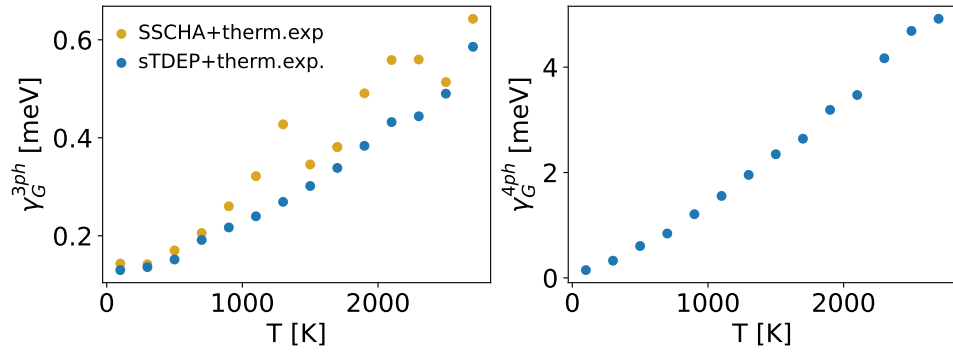

**Supplementary Figure 4.** Comparison between a three-phonon anharmonic contribution to the linewidth as obtained from SSCHA and from TDEP(SCHA) with a much larger four-phonon contribution obtained from TDEP(SCHA).

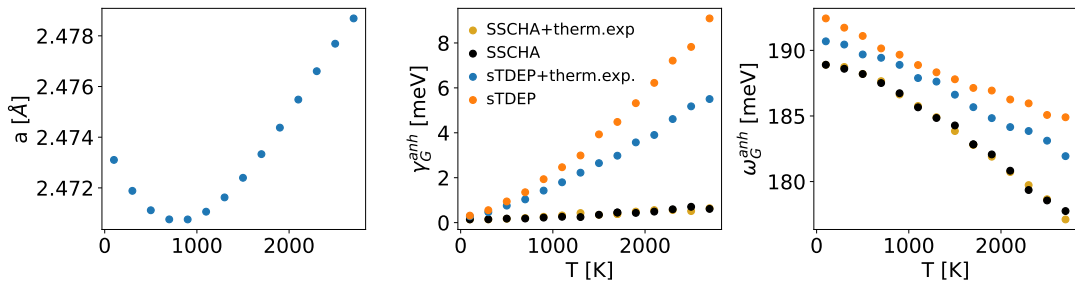

**Supplementary Figure 5.** In the first panel, we show the thermal expansion of the lattice constant. Comparison between a TDEP(SCHA) and SSCHA G mode linewidth and frequency calculation with and without the effects of thermal expansion.

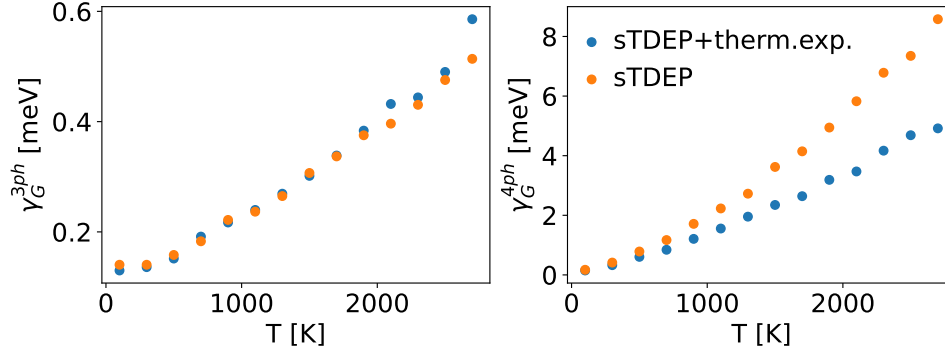

**Supplementary Figure 6.** Comparison between a three- and four-phonon contribution to the linewidth with and without thermal expansion as obtained from TDEP(SCHA). Thermal expansion effects are only noticeable in the four phonon contribution to the linewidth.

### Supplementary References

- [1] G. Montagnac, R. Caracas, E. Bobocioiu, F. Vittoz, and B. Reynard, “Anharmonicity of graphite from uv raman spectroscopy to 2700k,” *Carbon* **54**, 68–75 (2013).
- [2] Stéphane Berciaud, Melinda Y. Han, Kin Fai Mak, Louis E. Brus, Philip Kim, and Tony F. Heinz, “Electron and optical phonon temperatures in electrically biased graphene,” *Phys. Rev. Lett.* **104**, 227401 (2010).
- [3] H.-N. Liu, X. Cong, M.-L. Lin, and P.-H. Tan, “The intrinsic temperature-dependent raman spectra of graphite in the temperature range from 4k to 1000k,” *Carbon* **152**, 451–458 (2019).
- [4] Dong-Hun Chae, Benjamin Krauss, Klaus Klitzing, and Jurgen Smet, “Hot phonons in an electrically biased graphene constriction,” *Nano letters* **10**, 466–71 (2010).
